# Supplementary material for: EmphasisChecker: A Tool for Guiding Chart and Caption Emphasis
Source: arXiv:2307.13858 ancillary file (2024-01-20)
Supplement: Supplementary file 1 [file system-details.pdf]

# EmphasisChecker: A Tool for Guiding Chart and Caption Emphasis: Further Information on the Time-Series Prominent Feature Detector and Text References Extractor

## 1 Generated Features & Perception Study

As an alternate evaluation to the one described in the main paper, we performed a second test; we first combined the top-three features produced by the three methods (1) crowdsourced gold features [3], (2) EmphasisChecker features and (3) Contextifier features [2] to obtain up to nine features for each of the 43 charts (note that if these methods produced the same top feature we included it only once) (Figure 1). We then asked 8 participants per chart to rank all the features in the pool from most prominent to least prominent.

On average, the participants ranked 2.12 (70.5%) of the top three features generated by our method among the top three, whereas they ranked 1.95 (65.1%) of the crowdsourced features and 0.74 (24.5%) of the Contextifier features among the top three. This test further suggests that our approach outperforms Contextifier and is inline with the variance seen amongst human-labeled crowdsourced features.

## 2 $\varepsilon$-Persistence & Crowdsourced Prominence

the $\varepsilon$-persistence measure is roughly in line with the crowdsourced prominence ranking. The average $\varepsilon$-persistence of the crowdsourced most prominent feature, the crowdsourced second most prominent feature and the crowdsourced third most prominent feature are 0.146 ($\sigma = 0.105$), 0.094 ($\sigma = 0.092$) and 0.115 ($\sigma = 0.101$), respectively. We applied Friedman's tests for the rank-order data and then post-hoc Nemenyi's tests to examine pairwise comparisons [4]. Through the tests, we find that the difference between the most prominent and the second most prominent features is significant ($p = 0.030$), whereas the others are not statistically significant (most prominent-third most prominent: $p = 0.370$, second most prominent-third most prominent: $p = 0.463$). The reversal of the $\varepsilon$-persistence values between the second most prominent feature and the third most prominent feature is not surprising as the difference is insignificant and Kim et al. [3] also did not find significant difference in how they affect readers potentially due to their closeness in prominence.

## 3 Effects of Aspect Ratio on Prominent Features

When using our tool, the users can change a chart's aspect ratio by changing the chart's width and height as well as the x- and y- ranges. The use of Euclidean distances on the rendered chart allows our time-series prominent feature detector to capture changes of prominence of features depending on the aspect ratio (Figure 2).

## 4 Potential Artifacts of the RDP Algorithm

We note that when points near a local extremum or an inflection point have values close to the value of the local extremum/inflection point, the detected prominent point could be off by one or two points (e.g., Figure 3, second most prominent point off by a point from the minimum in 1987; Figure 3, most prominent point off by a point from the peak around March).

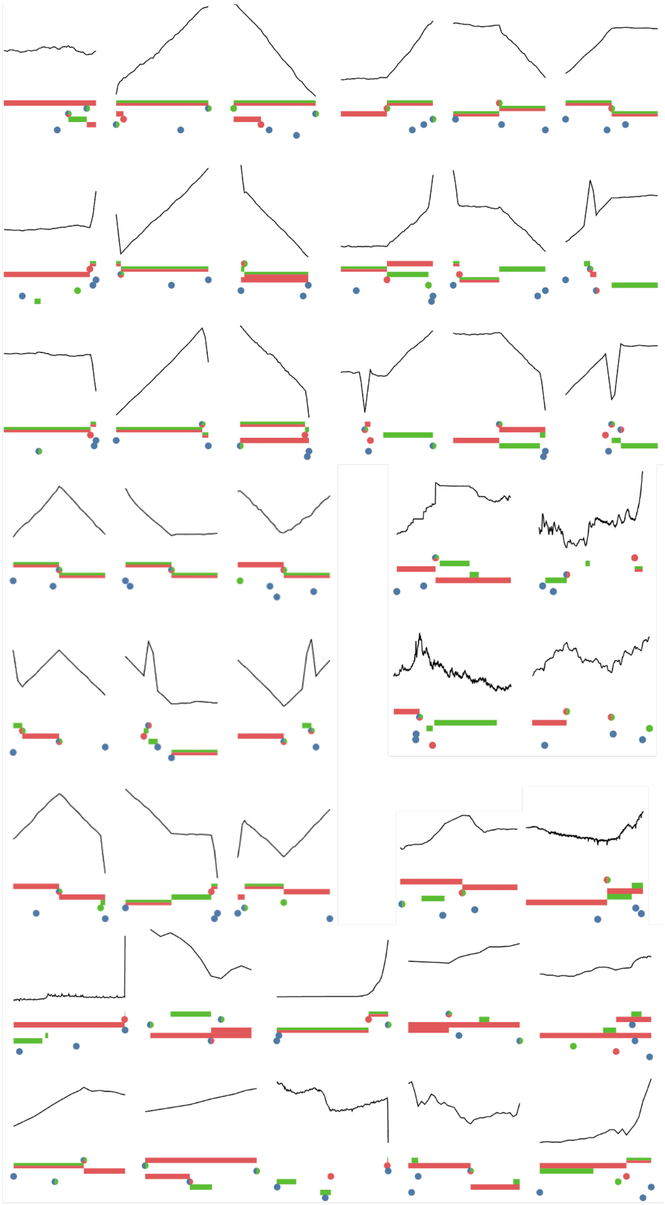

Fig. 1: Comparisons of the top three visually prominent features generated by (1) crowdsourcing [3] (green ■), (2) EmphasisChecker (red ■) and (3) Contextifier [2] (blue ■) on the 43 charts (synthetic and real-world) from Kim et al. [3]. Circles show point features and lines show trends. If two or more algorithms generated the same feature, we color the circle or line corresponding to the feature with multiple colors. The ordering of the features shows how often the participants of the perception study said that the feature is among the top three among these features.

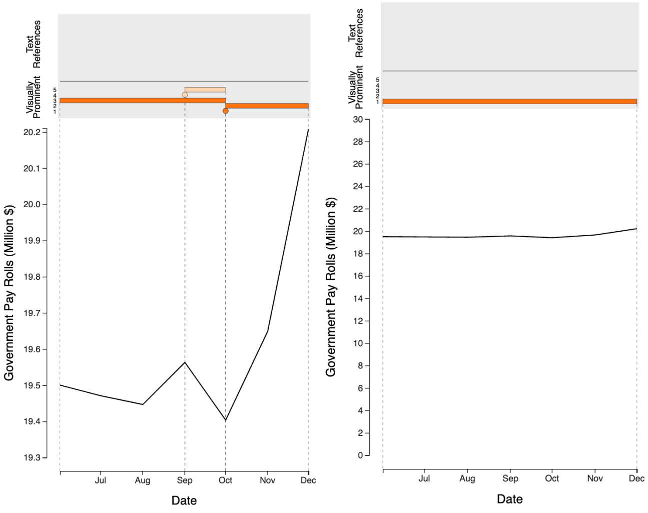


(a) *'Govt. Pay Rolls Up!'* (b) *'Govt. Pay Rolls Stable!'*

Fig. 2: Prominent feature detection results in the time-series line charts on government pay rolls in 1937 charts used as an example of how aspect ratios can change charts' messages in Huff [1]. The key message of each of the charts are shown as captions for each line chart, taken directly from the original source. The features EMPHASISCHECKER detects in each chart matches its key message. For (a), EMPHASISCHECKER detects the sudden increase starting in October as a feature of high prominence. For (b), EMPHASISCHECKER instead detects a single flat trend.

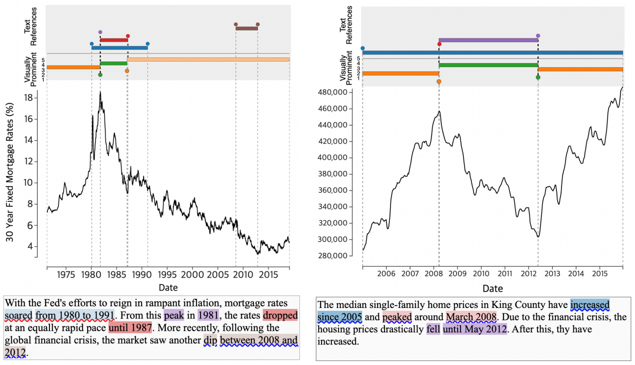


(a) Tourists inbound to Japan (b) North Korea's GDP per capita

Fig. 3: Artifacts of the RDP algorithm for charts and captions in (a) Figure 1 and (b) Figure 8d in the paper. (a) The second most prominent point feature is off by a point from the minimum in 1987. (b) The most prominent point feature is off by a point from the minimum in 1987.

## 5 TEXT REFERENCES DETECTOR ERROR ANALYSIS

On the 81 sentences collected through our user study, our text references detector correctly identified all references in 57 sentences (70%). It missed references and resulted in false negative (FN) errors in 22 sentences (27%), detected a non-existing reference and resulted in false positive (FP) errors in 4 sentences (5%), and extracted correct references based on the sentence but different from the author's intention resulting in intention mismatch errors (IM) errors in 2 sentences (2%) (4 sentences double-counted). Here, we describe two recurring error patterns we observed. Other unmentioned error patterns were present in only one or two sentences.

### 5.1 FN: No explicit time references / data descriptions (11 sentences)

The text references detector relies on the assumption that both time references and data descriptions are present within each sentence. Hence, when either the time reference or the data description is missing from the sentence, the text references detector fails to detect the reference and results in an FN error. Occasionally, the necessary information is available in previous sentences. For example, Figure 3b Sentence 3 includes the anaphoric reference *'this'*, which refers to *'May 2012'* in Sentence 2. As another example, one of the study participants wrote *'the trend reversed'* to refer to a trend mentioned in an earlier sentence. We also observed sentences that describe overall trends often omit the time reference (e.g., *"The tendency of the entire ratio is decreasing."*).

### 5.2 FN: Unhandled chart features (8 sentences)

In generating the word lists, we focused on detecting trends and extrema. Due to the limited scope of the word lists, descriptions of chart features that are not trends or extrema trigger FN errors. For example, some sentences referred to flat regions in the chart (e.g., *'stable'*, *'consistent'* or generic fluctuations (e.g., *'fluctuation'*, *'change'*).

## REFERENCES


[1] D. Huff. *How to Lie with Statistics*. W. W. Norton & Company, Inc., New York, USA, 1954. 2

[2] J. Hullman, N. Diakopoulos, and E. Adar. Contextifier: Automatic Generation of Annotated Stock Visualizations. In *Proceedings of the SIGCHI Conference on Human Factors in Computing Systems*, pp. 2707–2716. ACM, New York, USA, 2013. doi: 10.1145/2470654.2481374 1

[3] D. H. Kim, V. Setlur, and M. Agrawala. Towards Understanding How Readers Integrate Charts and Captions: A Case Study with Line Charts. In *Proceedings of the 2021 CHI Conference on Human Factors in Computing Systems*. 610. ACM, New York, USA, 2021. doi: 10.1145/3411764.3445443 1

[4] D. G. Pereira, A. Afonso, and F. M. Medeiros. Overview of Friedman's Test and Post-hoc Analysis. *Communications in Statistics - Simulation and Computation*, 44(10):2636–2653, 2015. doi: 10.1080/03610918.2014.931971 1
