# Supplementary material for: EmphasisChecker: A Tool for Guiding Chart and Caption Emphasis
Source: arXiv:2307.13858 ancillary file (2024-01-20)
Supplement: Supplementary file 2 [file survey-questions.pdf]

## List of the survey questions

1. Post-task reflection (Tool A)
    a. Part 1 of 3: Usefulness
        i. What messages did you intend to convey through your chart and caption? Any reason why you chose those messages? (If you need to, you may go back to the study screen)
        ii. How well do you think the readers will take away the message you wanted to convey?
        iii. Are there any messages readers viewing the chart and caption on paper (i.e., not interactive) might take away from the chart and caption other than the one intended? If so, what are they?
        iv. For each of the following statements about **Tool A**, please let us know how much you agree / disagree.
        v. The tool provides useful guides that are helpful when authoring charts and their captions.
        vi. The chart-caption pairs written with this tool will get the authors' messages well to the readers.
        vii. If any, what are the benefits of using this tool? Are there situations in which the tool would especially be useful?
        viii. If any, what are some downsides of this tool? Are there situations when the downsides would be especially pronounced?
        ix. Any other thoughts about the usefulness of this tool?
    b. Part 2 of 3: Usefulness
        i. I think that I would like to use this tool frequently.
        ii. I found the tool unnecessarily complex.
        iii. I thought the tool was easy to use.
        iv. I think that I would need the support of a technical person to be able to use the tool.
        v. I found the various functions in the tool were well integrated.
        vi. I thought there was too much inconsistency in the tool.
        vii. I would imagine that most people would learn to use this tool very quickly.
        viii. I found the tool very cumbersome to use.
        ix. I felt very confident using the tool.
        x. I needed to learn a lot of things before I could get going with this tool.
        xi. If any, what aspects of the tool were easy to use / intuitive?
        xii. If any, what aspects of the tool were difficult to use / counter-intuitive?
        xiii. Any other thoughts about the usability of the tool?
    c. Part 3 of 3: Free-Form Comments
        i. Any other thoughts about the tool that you would like to share with us?

2. Post-task reflection (Tool B)

a. Part 1 of 3: Usefulness
    i. What messages did you intend to convey through your chart and caption? Any reason why you chose those messages?
    ii. How well do you think the readers viewing the chart and caption on paper (i.e., not interactive) will take away the message you wanted to convey?
    iii. Are there any messages readers might take away from the chart and caption other than the one intended? If so, what are they?
    iv. The tool provides useful guides that are helpful when authoring charts and their captions?
    v. The chart-caption pairs written with this tool will get the authors' messages well to the readers.
    vi. If any, what are the benefits of using this tool? Are there situations in which the tool would especially be useful?
    vii. If any, what are some downsides of this tool? Are there situations when the downsides would be especially pronounced?
    viii. Any other thoughts about the usefulness of this tool?
b. Part 2 of 3: Usefulness
    i. I think that I would like to use this tool frequently.
    ii. I found the tool unnecessarily complex.
    iii. I thought the tool was easy to use.
    iv. I think that I would need the support of a technical person to be able to use the tool.
    v. I found the various functions in the tool were well integrated.
    vi. I thought there was too much inconsistency in the tool
    vii. I would imagine that most people would learn to use this tool very quickly.
    viii. I found the tool very cumbersome to use.
    ix. I felt very confident using the tool.
    x. I needed to learn a lot of things before I could get going with this tool.
    xi. If any, what aspects of the tool were easy to use / intuitive?
    xii. If any, what aspects of the tool were difficult to use / counter-intuitive?
    xiii. Any other thoughts about the usability of the tool?
c. Part 3 of 3: Free-Form Comments
    i. Any other thoughts about the tool that you would like to share with us?

3. EmphasisChecker Post-Survey
    a. EmphasisChecker Post-Survey (Part1 of 2): Tool Comparison
        i. Comparing Tool A and Tool B, which of the two is more useful when authoring charts and captions?
        ii. What is your rationale for your answer above?
        iii. Comparing Tool A and Tool B, which of the two is easier to use when authoring charts and captions?
        iv. What is your rationale for your answer above?

v. What other comparisons would you draw between Tool A and Tool B? In what ways is one better than the other?
vi. Anything else about the tools that you would like to share with us?

b. EmphasisChecker Post-Survey (Part 2 of 2): Free-Form Comments
   i. Any thoughts about the study that you would like to share with us?
   ii. Anything else you would like to share with us about?
