# Supplementary material for: EmphasisChecker: A Tool for Guiding Chart and Caption Emphasis
Source: arXiv:2307.13858 ancillary file (2024-01-20)
Supplement: Supplementary file 3 [file onboarding-instructions.pdf]

## Pre-Survey

---

Please complete the following pre-survey. Your ID for the pre-survey is:

writingWhiteFrog9705

Link to the survey: <https://forms.gle/kRGWKC8wj2waTDiM6>

After you finish, please input the completion code here (all lowercase):

Submit



## Preliminaries on Chart and Caption Emphasis

Take a look at the following chart from Pew Research, showing the number of U.S. citizens traveling internationally per month.

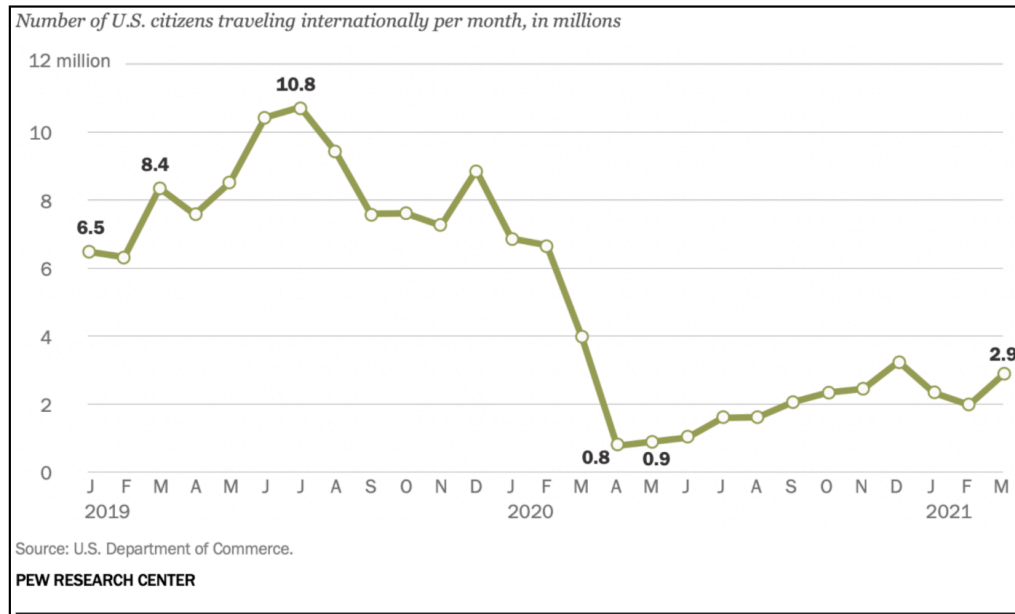

Take a moment to read each of the following captions and think about which of the following captions is the most effective in getting its message through when paired with this chart.

1. The chart shows the number of Americans traveling internationally each month since 2019. The x-axis shows years and ranges from January 2019 and March 2021. The y-axis shows the number of US citizens traveling internationally per month and takes on values between 0 and 12 million.
2. This graph about the number of Americans traveling internationally each month since 2019 shows the drastic effect of COVID-19 on US citizens traveling abroad. From its peak of 10.8 million in July 2019, the number of international travelers fell drastically down to its bottom of 0.8 million in April 2020. Since then, it has been on a slow recovery.
3. This is a graph about the number of Americans traveling internationally each month since 2019. The number of international travelers fell between January 2019 and February 2019 with the end of the winter holiday season. It recovered up to the summer vacation season around July 2019. It peaked again around December 2019, and again around December 2020 with the winter holiday season.

Q. Which of the captions above is the most effective in getting its message through when paired with the chart and why do you think so (briefly)?

Your answer here...

Next



## Preliminaries on Chart and Caption Emphasis

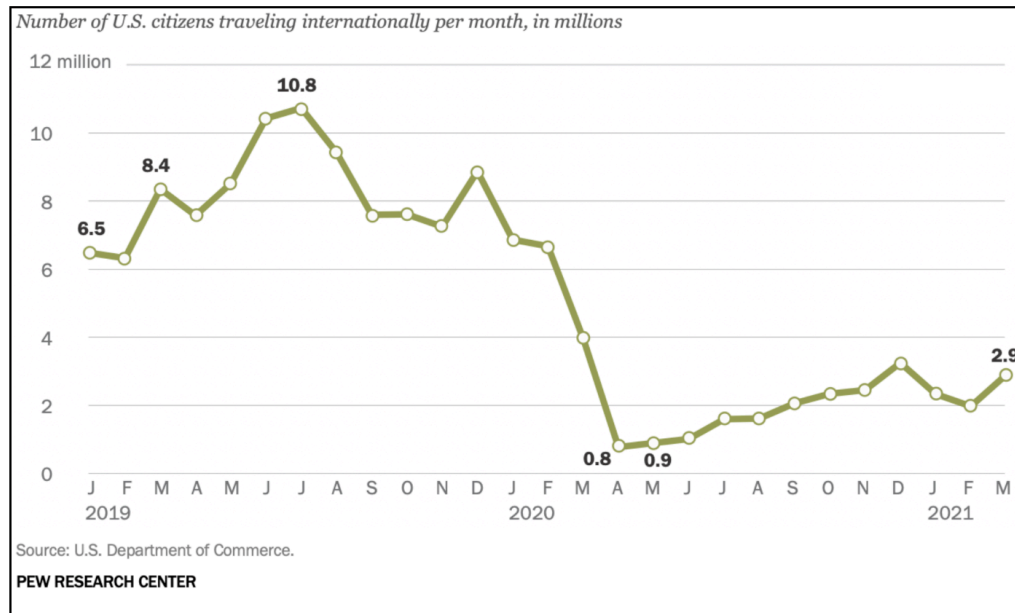

Here is our take on this question:

1. The chart shows the number of Americans traveling internationally each month since 2019. The x-axis shows years and ranges from January 2019 and March 2021. The y-axis shows the number of US citizens traveling internationally per month and takes on values between 0 and 12 million.

⇒ The first is a basic description only explaining how the chart encodes data and it may be unclear to the reader what the takeaway should be.

2. This graph about the number of Americans traveling internationally each month since 2019 shows the drastic effect of COVID-19 on US citizens traveling abroad. From its peak of 10.8 million in July 2019, the number of international travelers fell drastically down to its bottom of 0.8 million in April 2020. Since then, it has been on a slow recovery.

⇒ The second and third both describe specific features in the chart and covers various features throughout the chart, but we would argue that the second is better than the third because the second text has a better coverage of the **visually prominent features** of the chart, or in other words, what the reader would view as important in the chart, although it does skip over some less significant features.

3. This is a graph about the number of Americans traveling internationally each month since 2019. The number of international travelers fell between January 2019 and February 2019 with the end of the winter holiday season. It recovered up to the summer vacation season around July 2019. It peaked again around December 2019, and again around December 2020 with the winter holiday season.

⇒ What the third caption says is factually correct, but it does not really describe the visually prominent features.

Next



## Preliminaries on Chart and Caption Emphasis

---

To help you write more effective text about the charts, we built ***EmphasisChecker***, a tool that helps you align the message in your text with the message in the chart by displaying the visually prominent features in the chart and the references to the chart in the text.

Next



## Instructions: Uploading data

Once you begin, you would need to either:

- select one of the provided data by using the dropdown menu on the left, or
- upload your own data by either clicking the region on the right or drag-dropping the data into the region.

Choose one of the default charts:

16 ▾

OR

Upload your own data:

Drop your data file here (.csv)  
OR  
Click here to upload your data file

Note: If you are uploading your own data, please ensure that the file is in the right format. The file should be in a CSV format with the first column named "Date" and the second column giving the description of the values. The first column should include dates of the form "YYYY-MM-DD" and the second column should include the either integers or decimals.

If you see nothing happening for a while, it means that the file is not in the right format. Please reformat your data or use one of the provided data if you run into this issue.

Next



Instructions: Tool A vs. Tool B

After you upload the data, you will be directed to a chart-caption authoring interface, either Tool A or Tool B.

The two interfaces look like the following:

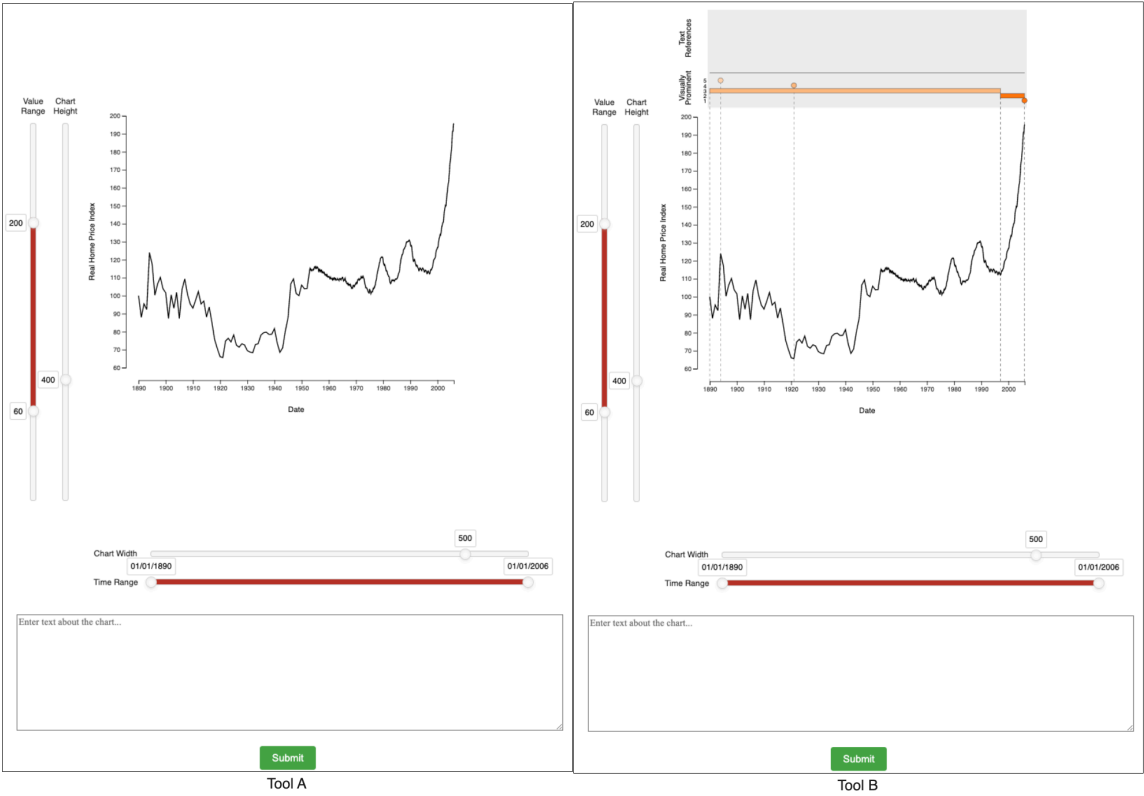

Note that the key difference between the two interfaces is the gray panel on top of the chart that shows the chart's visually prominent features and text references to chart features.

Next



## Instructions: Tool A and B Authoring Interface

In either case, you will use the interface to make changes to the chart and the caption while exploring the data.

For the chart, you will be able to change the ranges of time and value and the dimensions of the chart using the sliders to the left and the bottom of the chart.

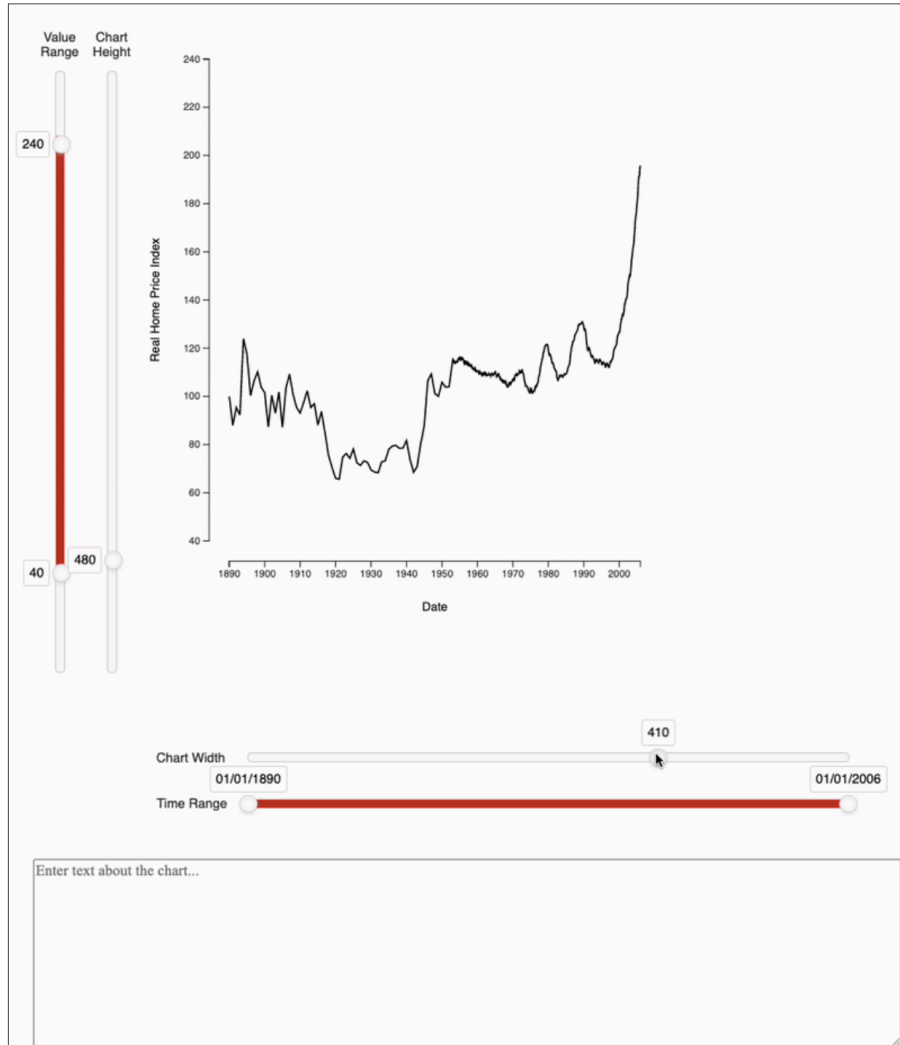

Next



## Instructions: Tool A and B Authoring Interface

You can also hover your mouse over the chart navigate through the chart and read off values.

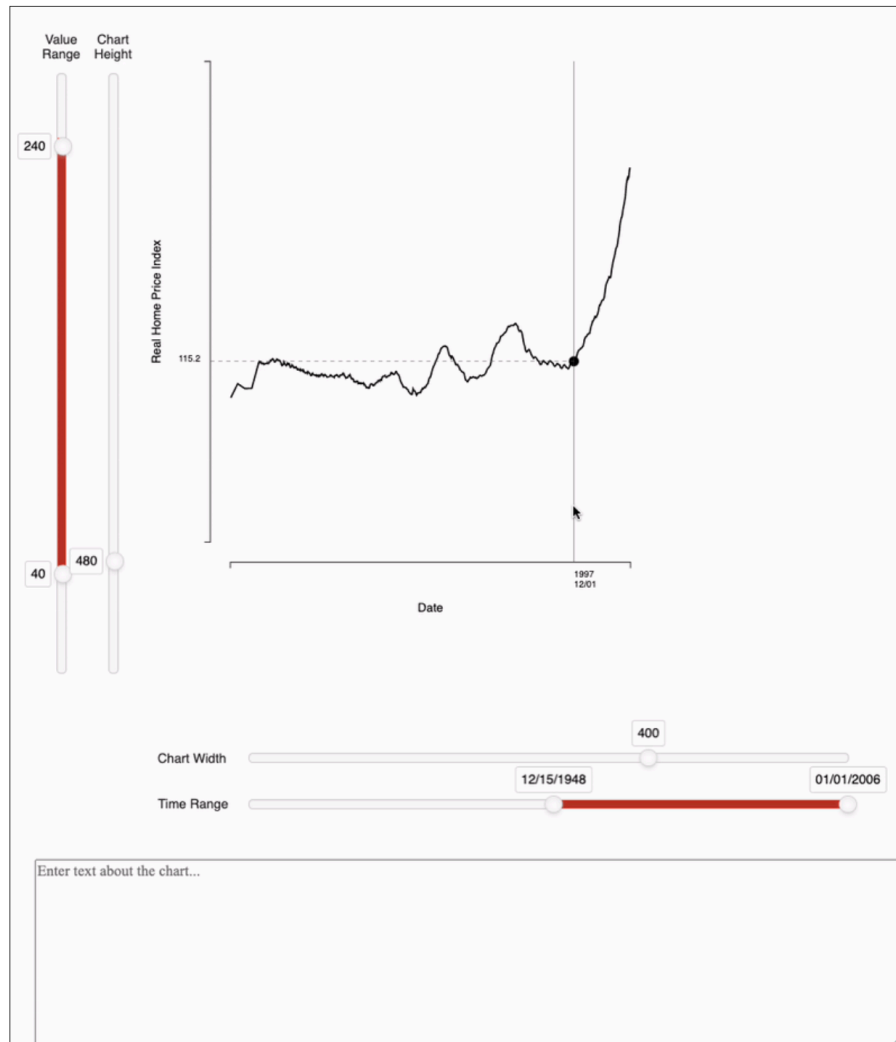

Next



## Instructions: Tool A and B Authoring Interface

You would write the caption in the text box below the chart.

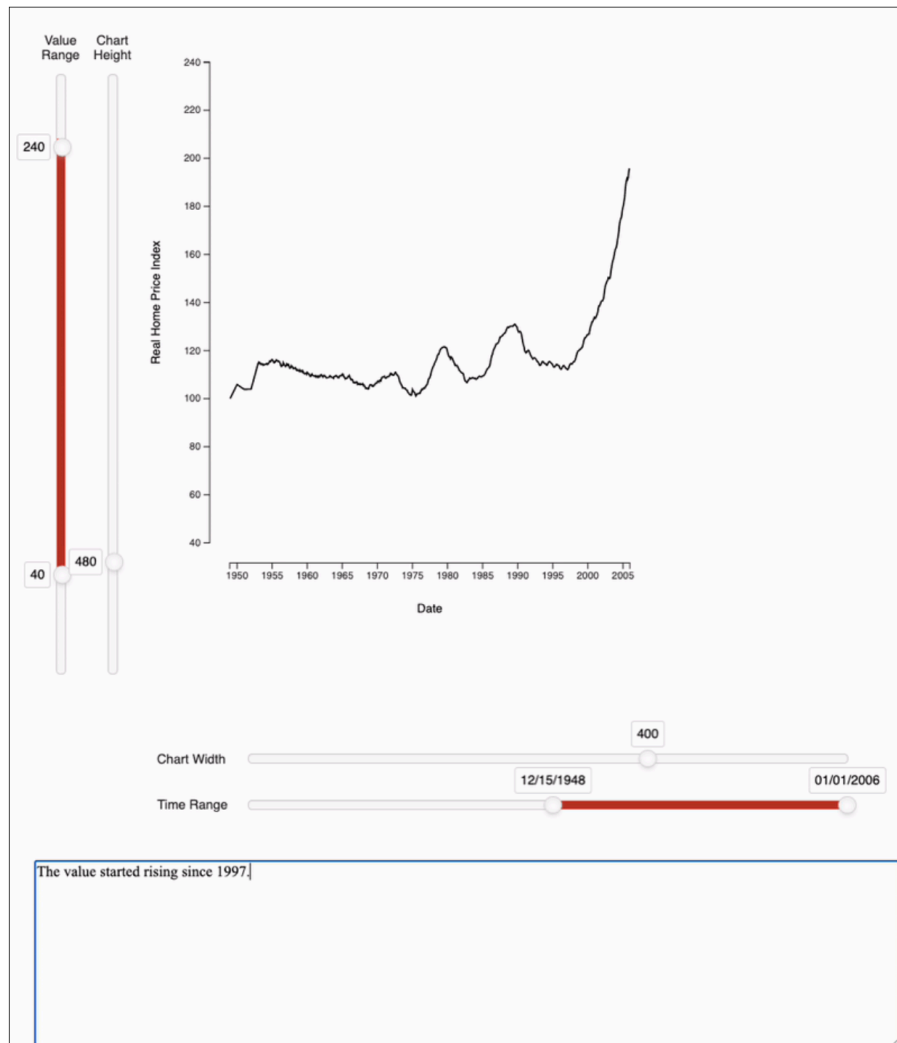

Note that you may go back and forth between these functionalities as you feel necessary. For example, you can resize the chart and change the time range while writing the caption or after writing the caption.

Next



## Instructions: Tool B Additional Features

When you have access to Tool B, you will immediately see some orange bars and circles above the chart. These show the locations of the chart's top five visually prominent features (i.e., chart emphasis) based on Tool B's analysis, with the most prominent closest to the bottom.

You may or may not agree with the Tool B's analysis of the visually prominent features as visual prominence is a subjective matter.

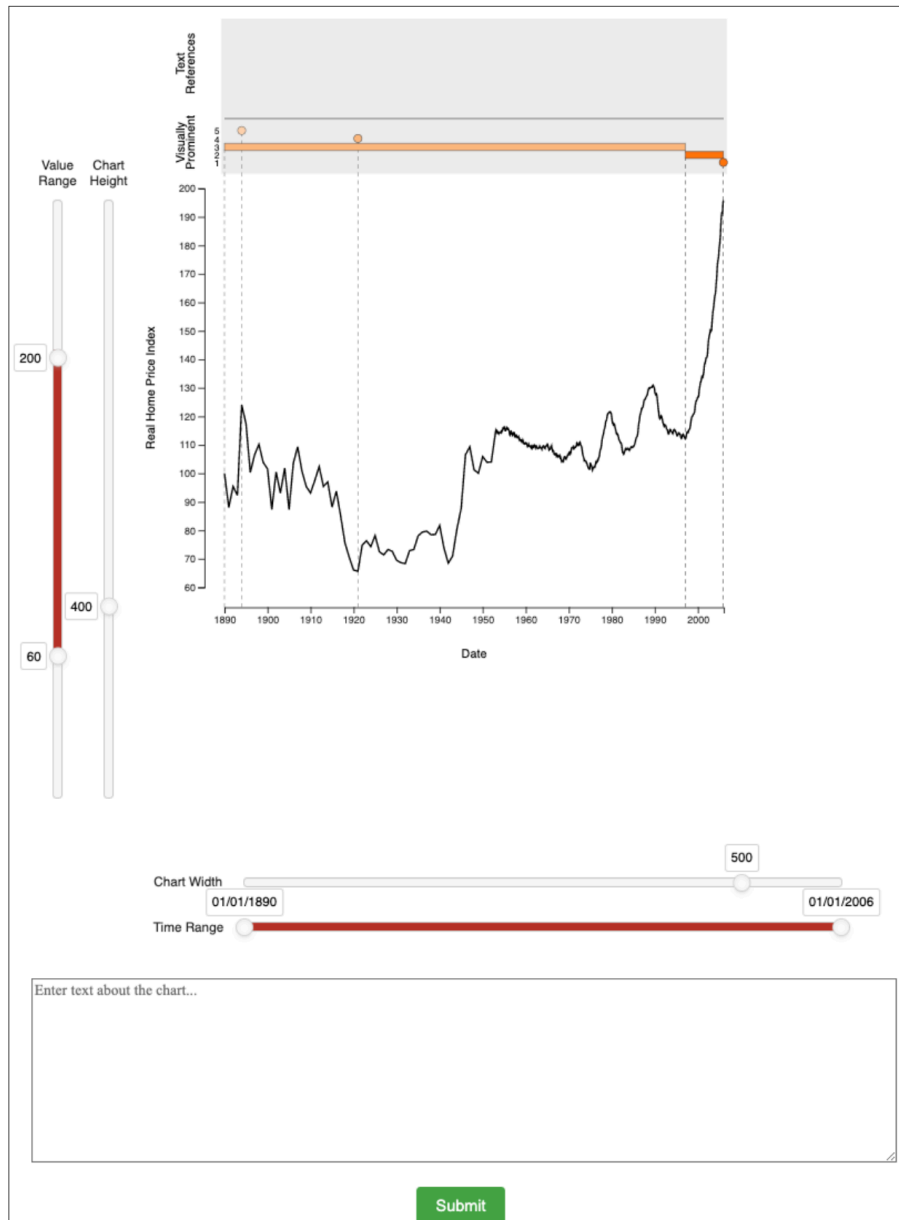

You should observe that the chart's prominent features depends on your the choice of time and value ranges as well as the dimensions of the chart.

Next



## Instructions: Tool B Additional Features

During authoring, you can press **SHIFT + ENTER** to invoke Tool B's emphasis analysis.

Once you press SHIFT+ENTER, the parts of the text that refer to portions of the chart's features (i.e., text emphasis) will be highlighted and will be shown in the gray box above the visually prominent features display (blue in this example). Here, the rising trend since 1997 is captured along with the starting point of the trend, which is explicitly mentioned in the caption.

The visually prominent features matched by the text emphasis will be highlighted in green.

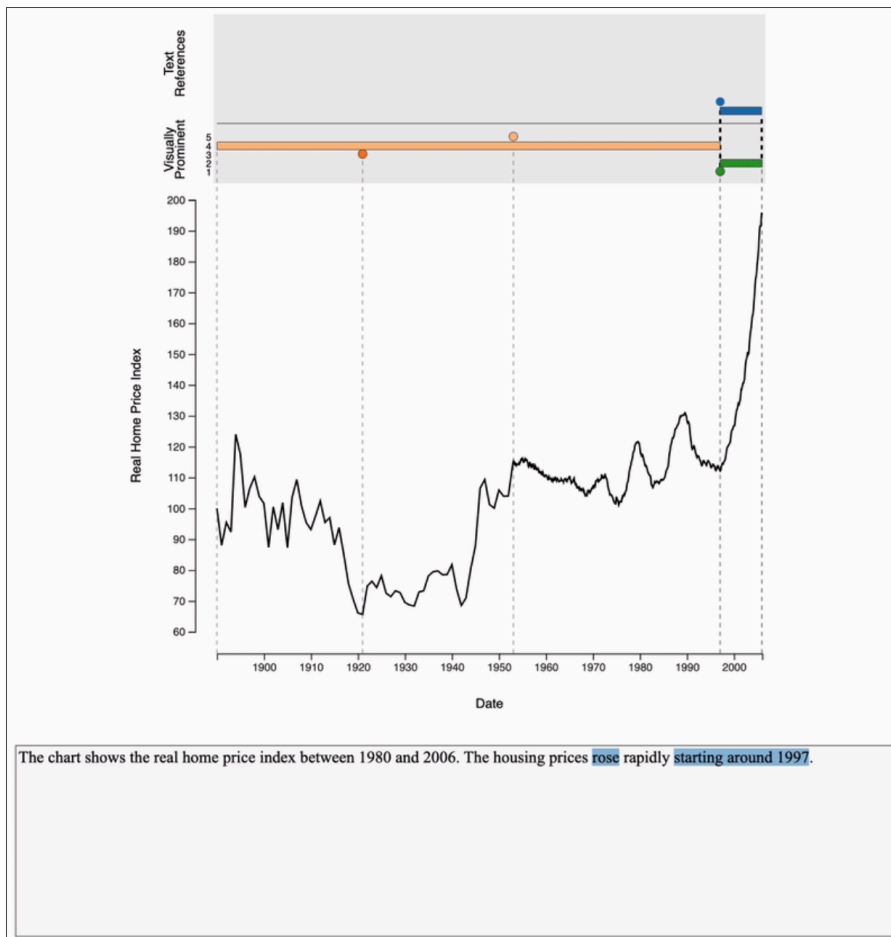

Next



## Instructions: Tool B Additional Features

Sometimes, Tool B will detect potential issues with the caption and will mark the text. There are two types of potential issues that EmphasisChecker can notify you of:

- Red squiggly: Potential factual errors
- Blue squiggly: Text potentially describing insignificant chart feature

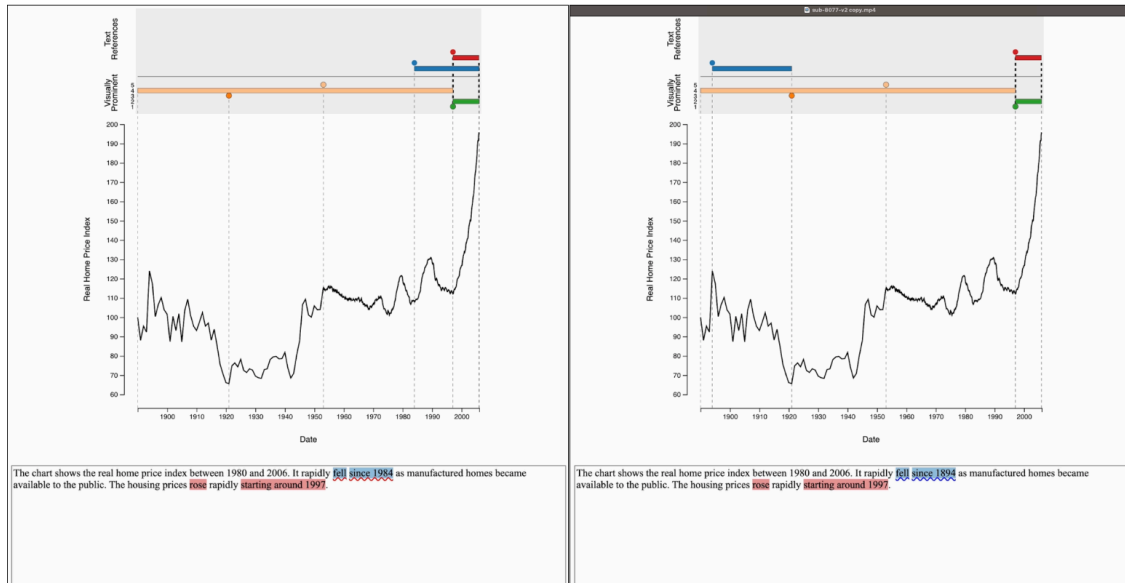

Red squiggly underline under 'fell since 1984'. This is a factual error since the values actually 'rose since 1984'.

Blue squiggly underline under 'fell since 1894'. Tool B does not recognize the fall since 1894 as visually prominent.

Remember: Tool B is only **suggesting potential issues** and you might not agree with its analysis.

***It is ultimately up to you to decide whether to accept or reject the suggestions.***

Next
